# Supplementary material for: Car that Knows Before You Do: Anticipating Maneuvers via Learning Temporal Driving Models
Source: arXiv:1504.02789 source file (2015-09-19)
Supplement: Supplementary file 1 [file model_supplementary.tex]

\section{Approach}
\begin{figure}
\centering
\includegraphics[width=\linewidth]{../Fig/model}
\caption{AIO-HMM}
\label{fig:model}
\end{figure}

We first describe our model for anticipating maneuvers. Following this we
explain multi-modal context features and the inference algorithm.

\subsection{Context for anticipating maneuvers}
Driving maneuvers occur due to multiple interactions that may include the driver,
the vehicle, nearby traffic and sometimes also the driver's destination. 
In order to anticipate maneuvers we have to model these
interactions in a tractable manner and identify useful sources
of information for these interactions. 
Information from inside the car is useful
for infering drivers intention. Drivers physical posture such as their head
movement provides strong cues of their intented maneuver. For example, prior to a
maneuver drivers reveal their intention by scanning their surrounding for
traffic. This context should be further augmented
with outside-vehicle information. We now describe the features we extract for
anticipation. 
\\~\\~
\noindent \textbf{Inside-vehicle context features.} Our inside-vehicle features captures drivers head movement. Our autonomous vision pipeline
consist of face detection, tracking and feature extraction
modules. 

\noindent \textit{Face detection and tracking.} We detect
driver's face using trained Viola-Jones face detector~\citep{Viola04}. On the detected face
we find visually discriminative points using Shi-Tomasi corner
detector~\citep{Shi94} and track the detected points using
Kanade-Lucas-Tomasi tracker~\citep{Lucas81,Shi94,Tomasi91}. However, tracking
may accumulate error over time because of changes in illumination due to shadows
of the trees, 
traffic, etc. Thefore, we constraint the tracked points to follow a projective transformation
and remove incorrects tracks using RANSAC. After every frame we loose some of
the tracked points. We re-initialize the tracker with new corner points
once old points falls below a threshold~\citep{Kalal10}. \todo{Our tracking results
with some failure cases are available here:}

\noindent \textit{Features from face track.} 
For anticipation horizontal movement of face and its angular
rotation (\textit{yaw}) are particularly important. 
From face tracking we obtain many 2D trajectories in the image plane 
corresponding to the movement of facial points (\todo{Figure}~\ref{fig:face_move}). We
represent facial movements and rotations with histrogram features. 
In particular we take matching points between successive frames and create
histograms for pixels horizontal and angular motion in the image plane. We bin
horizontal and angular motion between successive frames using $[\leq-2,\;-2\;\text{to}\;0,\;0\;\text{to}\;2,\;\geq2]$ and  
$[0\;\text{to}\;\frac{\pi}{2},\;\frac{\pi}{2}\;\text{to}\;\pi,\;\pi\;\text{to}\;\frac{3\pi}{2},\;\frac{3\pi}{2}\;\text{to}\;2\pi]$
bins,
respectively. We also calculate mean movement of the center of face. This gives
us $\phi(\text{face})\in\mathbb{R}^9$ facial features for each frame.

We denote inside-vehicle features with $I$. For AIO-HMM we accumulate and
normalize $\phi(\text{face})$ for every 20 frames. Thus, $I =
\sum_{i=1}^{20}\phi(\text{face}_i)/\|\sum_{i=1}^{20}\phi(\text{face}_i)\|$ for
AIO-HMM.
\\~\\~
%\subsection{Outside-vehicle context features}
\noindent \textbf{Outside-vehicle context features.} The outside environment such as road conditions, vehicle speed, traffic etc.,
influence drivers intention for maneuvers, and affects their physical
state such as head movement, facial expressions etc. For example,
intersections and turns influence the driver to move head to scan for the cross traffic. 
Simiarly, while driving in the farthest lanes head movements indicating lane changes are less likely.

We combine information from road facing camera with speed and GPS coordinates of the
vehicle. Using the outside camera we obtain two binary
features  indicating whether lanes exist on either side of vehicle. We
augment GPS coordinates with map information and extract a binary feature to
indicate approaching
intersections and turns. Speed of the vehicle also influence drivers mental
state. Maneuvers such as turns are generally performed at lower speeds.
We use average, maximum and minimum speed of the car over 5 seconds as features. 
This results in $\phi(\text{outside})\in\mathbb{R}^6$ dimensional feature vector. 
For every $\phi(\text{face})$ we extract $\phi(\text{outside})$. We denote
outside features with $O$.

\subsection{Modeling driving maneuvers}
Modeling maneuvers essentially requires temporal modeling of inside and outside
vehicle context. Temporal aspect of the problem is critical because informative cues such
as drivers head movement occurs at variable time before maneuver
(\todo{Figure}~\ref{fig:time_variance}). Discriminative
methods such as Support Vector~\citep{Cortes95} and Relevance Vector
Machines~\citep{Tipping01} ignores this temporal aspect and therefore performs poorly.

Temporal models such as Hidden Markov Models (HMM)~\citep{Rabiner86} are better
suited for this problem. HMM introduce parameters for 
\textit{hidden} mental state $Z$ of driver and models how $Z$ generates
observations $I$
and $O$. 
%Assuming drivers have some \textit{hidden} mental state $Z$ that correlates with 
%observations $I$ and $O$. 
%HMM models how the mental state $Z$ generates observations
%$I$ and $O$. 
However, the reasoning modeled by HMM is incorrect. In practice, it
is the events outside the vehicle $O$ that affects mental state $Z$ of driver which
further generates inside vehicle observations $I$. Therefore, 
interactions between $O$ and $Z$ needs discriminative modeling, and a generative
model between $Z$ and $I$.
Input-Output HMM
(IOHMM)~\citep{Bengio95} models this behaviour. However, it does not
model temporal dependencies of observations. We model observation dependencies because
human face movements are smooth and temporally correlated. Our model is
therefore called Autoregressive Input-Output HMM (AIO-HMM) as shown in
\todo{Figure}~\ref{fig:model}.

\section{Learning Algorithm}
\todo{Then talk about HMM and IOHMM and why we need AIO-HMM. After this talk
about learning algorithm.}

\subsection{Modeling maneuvers with Autoregressive Input-Output HMM (AIO-HMM)}

Given driving context $\mathcal{C}$, $t$ seconds before occurence of maneuver
$M$. The goal is to learn a model $P(\mathcal{C}|M)$. The context $\mathcal{C} =
\{\mathcal{O};\mathcal{I}\}$ is further
divided in two parts: (i) outside-vehicle $\mathcal{O}$; and (ii) inside-vehicle
$\mathcal{I}$
contexts. We also model driver hidden mental state $\mathcal{Z}$ while performing the maneuver.

$$P(\mathcal{C}|M) = \sum_\mathcal{Z} P(\mathcal{C},\mathcal{Z}|M) \propto
\sum_\mathcal{Z} P(\mathcal{I},\mathcal{Z}|\mathcal{O},M)$$  

We propose an autoregressive input-output HMM (AIO-HMM) to model $P(\mathcal{C}|M)$.
Our AIO-HMM is an extension of input-output HMM by Bengio et
al.~\citep{Bengio95} to handle dependencies in observations. Figure~\ref{fig:model} shows the AIO-HMM model. Because informative
cues can occur anywhere in the $t$ seconds of context $\mathcal{C}$, we divide
$\mathcal{C}$ into $T$
chunks (0.8 sec/chunk) and denote features of chunk $i$ with $C_i = \{O_i,I_i\}$.
At time instant $i$ drivers
mental state is $Z_i$, inside and outside context features are $I_i$ and
$O_i$ respectively. $I_i$ and $O_i$ are vectors and $Z_i$ is discrete state.

The input (top) layer of AIO-HMM consist of 
outside-vehicle context features $O_1^T = \{O_1,..,O_T\}$. The hidden (middle) layer represents
drivers mental state $Z_1^T = \{Z_1,..,Z_T\}$, and the
output (bottom) layer is the inside-vehicle context features such as divers head
movement before the maneuver $I_1^T = \{I_1,..,I_T\}$. AIO-HMM captures the relation that
outside-vehicle environment influence drivers mental state to perform the
maneuver, 
which then generates the inside-vehicle features. Our model is autoregressive
because successive inside-vehicle features are correlated due to short
duration (0.8 sec) chunks. We should also note that AIO-HMM does not make any
assumptions on the time of occurence of informative cues before the maneuver. In
fact the cues can appear anywhere within the time interval $t$.  

\subsection{AIO-HMM parameter estimation}
\noindent \textbf{\textit{M-step:}} We update the parameters
$\boldsymbol\Theta = \argmax_{\boldsymbol\Theta}
Q(\boldsymbol\Theta;\boldsymbol\hat{\boldsymbol\Theta})$. For
parameters $\boldsymbol\mu$, $\mathbf{a}$, $\mathbf{b}$ and
$\mathbf{\Sigma}$ we find closed form update expressions, and update
$\mathbf{w}$ using gradient decent. Before giving the update equations we define
shorthand $c_{it} = 1 + \mathbf{a}_i \cdot O_t + \mathbf{b}_i \cdot I_{t-1}$,
such that $\boldsymbol\mu_{it} = c_{it}\boldsymbol\mu_{i}$.
$$\boldsymbol\mu_{i} = \frac{\sum_{p=1}^N
\sum_{t=1}^{T_p}c_{it}\gamma_{it}I_{t}}{\sum_{p=1}^N \sum_{t=1}^{T_p}c_{it}^2\gamma_{it}}$$

$$\mathbf{\Sigma}_i = \frac{\sum_{p=1}^N\sum_{t=1}^{T_p}\gamma_{it}(I_tI_t^T +
c_{it}^2\boldsymbol\mu_{i}\boldsymbol\mu_{i}^T - c_{it}I_t\boldsymbol\mu_{i}^T-
c_{it}\boldsymbol\mu_{i}I_t^T)}{\sum_{p=1}^N \sum_{t=1}^{T_p}\gamma_{it}}$$

$$\mathbf{a}_i=\left[\sum_{p=1}^N \sum_{t=1}^{T_p}\gamma_{it}O_tO_t^T\right]^{-1}\sum_{p=1}^N\sum_{t=1}^{T_p}\gamma_{it}\left[\frac{O_tI_t^T\mathbf{\Sigma}_i^{-1}\boldsymbol\mu_i}{\boldsymbol\mu_i^T\mathbf{\Sigma}_i^{-1}\boldsymbol\mu_i}-O_t-O_{t}I_{t-1}^T\mathbf{b}_i\right]$$

$$\mathbf{b}_i=\left[\sum_{p=1}^N
\sum_{t=1}^{T_p}\gamma_{it}I_{t-1}I_{t-1}^T\right]^{-1}\sum_{p=1}^N\sum_{t=1}^{T_p}\gamma_{it}\left[\frac{I_{t-1}I_t^T\mathbf{\Sigma}_i^{-1}\boldsymbol\mu_i}{\boldsymbol\mu_i^T\mathbf{\Sigma}_i^{-1}\boldsymbol\mu_i}-I_{t-1}-I_{t-1}O_{t}^T\mathbf{a}_i\right]$$
\todo{Write vision features, talk about the pipeline}

\subsection{How we make the prediction.}
